# Supplementary material for: Modeling Target-side Inflection in Placeholder Translation
Source: arXiv:2107.00334 source file (2021-07-01)
Supplement: Supplementary file 1 [file appendix.tex]

\section{Corpus Statistics}
\begin{table}[]
\begin{tabular}{cccc}
train                       & augmented train data        & validation               & test                     \\
\multicolumn{1}{r}{996,877} & \multicolumn{1}{r}{199,080} & \multicolumn{1}{r}{1480} & \multicolumn{1}{r}{1456}
\end{tabular}
\end{table}
